# Supplementary material for: Task-Oriented GNNs Training on Large Knowledge Graphs for Accurate and Efficient Modeling
Source: arXiv:2403.05752 source file (2024-03-22)
Supplement: Supplementary file 1 [file appendix.tex]

\section{Appendix}
\label{sec:appendix} 
\begin{figure*}[h]
  \centering
   \includegraphics [width=\textwidth,height=10cm]{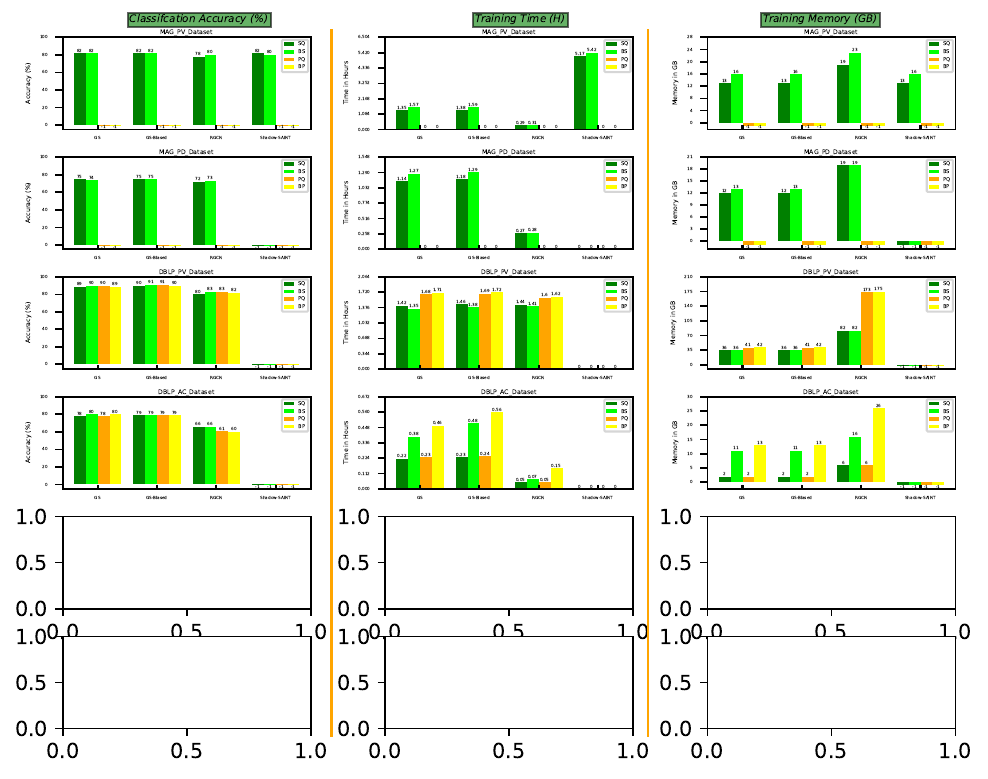}
  \caption{ (a) the accuracy, (b) the training time, and (c) training memory of node classification task using Graph-SAINT (GS) and RGCN on the three knowledge graphs including( DBLP, MAG, Yago4). 
  % Different data sets were extracted from the KGs and were used for the evaluation namely (RG: Relevant sub-graph, FG: Full Graph, and SQ: Star-Query Sub-graph). 
  The  {\sysName} tasked based samplers (SQ vs BS vs PQ vs BP)  }
%   BSG: Biased sampled sub-graph, GSG: Genetic selected Sub-graph, SQ: Star-Query Sub-graph, B-SQ: Bidirectional Star-Query Sub-graph, PQ: Path-Query Sub-graph, B-PQ: Bidirectional Path Query Sub-graph). The Star query Subgraph using GraphSAINT classifier achieves the highest accuracy with minimal resources. }
  \label{fig:TOSA_Samplers_Results}
    \ncp\ncp\ncp\ncp
\end{figure*}
\begin{table*}[!htp]\centering
\caption{GNN training pipeline steps including the role, techniques used, and challenges for each step}\label{tbl_GNN_pipeline}
\scriptsize
\begin{tabular}{|p{5em}|p{10em}|p{10em}|p{14em}|p{14em}|p{10em}|p{6em}|}
\toprule
\multirow{2}{} 
&\multirow{2}{50}{Graph Data Store} &\multicolumn{3}{c|}{Dataset ETL} &\multicolumn{2}{c|}{Graph ML} \\\cmidrule{3-7}
& &Dataset Extraction &Dataset Transformation & Dataloader &Training &Inferencing \\
\midrule
Role &Storing and maintaining graph data &Extract subgraph or a whole graph dataset & Automates dataset processing and splitting, to provide graph objects (vertices and relations) in adjacency matrix format &Load graph data into memory and convert it into sparse-matrics &Training GNN model &Predict nodes/edges \\
% \hline
Technique &Virtuoso, Jena,.. etc &KG Quering Languages i.e SPARQL, Cypher, etc. &Pandas data frames &Pytorch sparse matrix &full-graph or sample-based training. &Node classification Link prediction \\
% \hline
challenges &supporting machine learning on top of KG i.e providing ML learning operators on a form of SPARQL operators &retrieve graph dataset in a tabular format &Data format be compatible with PyTorch and its associated graph libraries i.e PyTorch Geometric \cite{PyGeometric}, and Deep Graph Library \cite{DistDGL} &Compressed sparse metrics that fit limited memory & better generalization and lower resources (Training time and memory) &Inductive Deductive \\
\bottomrule
\end{tabular}
\end{table*}
\begin{table*}
\centering
\caption{KGTOSA-Samplers Results}\label{tab: }
\scriptsize
\begin{tabular}{|l|r|rrrrrr|rrrrrr|rrrrrrr|}
\toprule
\multirow{2}{*}{\textbf{Dataset}} &\multirow{2}{*}{\textbf{Method}} &\multicolumn{6}{c}{\textbf{Accuracy(\%)}} &\multicolumn{6}{c}{\textbf{Training Time (Hours)}}&\multicolumn{6}{c}{\textbf{Training Memory (GB)}} \\\cmidrule{3-20}
& &\textbf{RS} &\textbf{FG} &\textbf{SQ} &\textbf{BS} &\textbf{PQ} &\textbf{BP} &\textbf{RS} &\textbf{FG} &\textbf{SQ} &\textbf{BS} &\textbf{PQ} &\textbf{BP} &\textbf{RS} &\textbf{FG} &\textbf{SQ} &\textbf{BS} &\textbf{PQ\_} &\textbf{BP} \\\midrule
\multirow{4}{*}{MAG\_PV} &GS &46.51 ± 0.47 &-1 & 82.50 ± 0.12 &82.35 ± 0.13 &-1 &-1 &0:58:29 &-1 &1:20:45 &1:34:17 &-1 &-1 &12 &-1 &13 &16.6 &-1 &-1 \\
&GS-Biased &47.55 ± 0.44 &-1 & 82.70 ± 0.12 &82.50 ± 0.10 &-1 &-1 &0:59:29 &-1 &1:22:45 &1:35:17 &-1 &-1 &12 &-1 &13 &16.6 &-1 &-1 \\
&RGCN & 36.79 ± 0.64 &-1 &78.08 ± 1.40 &80.23 ± 1.48 &-1 &-1 &0:09:10 &-1 &0:17:34 &0:18:30 &-1 &-1 &19 &-1 &19.7 &23.4 &-1 &-1 \\
&Shadow-SAINT &40.78 ± 0.15 &-1 &82.15 ± 0.55 &80.23 ± 1.48 &-1 &-1 &2:15:00 &-1 &5:10:14 &5:25:14 &-1 &-1 &12.8 &-1 &13.5 &16.9 &-1 &-1 \\
\midrule
\multirow{4}{*}{MAG\_PD} &GS &70.15 ± 0.54 &-1 &75.05 ± 0.09 &74.50 ± 0.32 &-1 &-1 &0:31:40 &-1 &1:08:30 &1:16:09 &-1 &-1 &11 &-1 &12.5 &13 &-1 &-1 \\
&GS-Biased & 70.34 ± 0.09 &-1 &75.68 ± 0.07 &75.19 ± 0.30 &-1 &-1 &0:32:40 &-1 &1:10:30 &1:17:09 &-1 &-1 &11 &-1 &12.5 &13 &-1 &-1 \\
&RGCN &68.83 ± 0.34 &-1 &72.33 ± 0.78 &73.08 ± 0.58 &-1 &-1 &0:07:00 &-1 &0:16:14 &0:16:44 &-1 &-1 &15.8 &-1 &19.2 &19.9 &-1 &-1 \\
&Shadow-SAINT &-1 &-1 &-1 &-1 &-1 &-1 &-1 &-1 &-1 &-1 &-1 &-1 &-1 &-1 &-1 &-1 &-1 &-1 \\
\midrule
\multirow{4}{*}{DBLP\_PV} &GS &58.15 ± 0.14 & 81.79 ± 0.26 &89.88 ± 0.30 &90.42 ± 0.47 &90.85 ± 0.65 &89.98 ± 0.43 &0:15:23 &1:51:24 &1:25:15 &1:21:16 &1:40:54 &1:42:29 &9 &46.6 &36 &36.5 &41 &42.5 \\
&GS-Biased & 58.39 ± 0.29 &80.53 ± 1.37 &90.00 ± 1.47 &91.45 ± 0.58 &91.36 ± 0.99 & 90.28 ± 0.90 &0:17:23 &1:54:24 &1:27:48 &1:22:35 &1:41:23 &1:43:15 &9 &46.6 &36 &36.5 &41 &42.5 \\
&RGCN & 53.30 ± 1.15 &74.16 ± 0.87 &80.07 ± 1.25 &83.23 ± 2.03 &83.44 ± 3.64 &82.74 ± 2.61 &0:08:23 &1:58:10 &1:26:32 &1:24:42 &1:35:48 &1:37:18 &12.3 &220 &82 &82.6 &173 &175 \\
&Shadow-SAINT &-1 &-1 &-1 &-1 &-1 &-1 &-1 &-1 &-1 &-1 &-1 &-1 &-1 &-1 &-1 &-1 &-1 &-1 \\
\midrule
\multirow{4}{*}{DBLP\_AC} &GS &33.08 ± 9.45 &80.79 ± 0.45 &78.88 ± 1.30 & 80.22 ± 0.12 &78.87 ± 0.59 &80.05 ± 0.36 &0:03:47 &2:49:34 &0:12:57 &0:23:00 &0:14:04 &0:27:38 &1.1 &79.8 &2.7 &11.4 &2.9 &13.2 \\
&GS-Biased & 33.05 ± 1.10 &85.07 ± 0.27 &79.26 ± 0.58 & 79.31 ± 0.86 &79.16 ± 0.32 &79.26 ± 0.54 &0:05:05 &2:57:00 &0:14:05 &0:28:57 &0:14:24 &0:33:32 &1.1 &79.8 &2.7 &11.4 &2.9 &13.2 \\
&RGCN & 40.90 ± 0.20 &75.86 ± 0.53 &66.07 ± 2.40 &66.80 ± 3.83 &61.59 ± 2.61 & 60.71 ± 0.70 &0:00:30 &2:13:46 &0:02:43 &0:04:14 &0:02:43 &0:08:54 &1.4 &207 &6 &16.7 &6.2 &26.7 \\
&Shadow-SAINT &-1 &-1 &-1 &-1 &-1 &-1 &-1 &-1 &-1 &-1 &-1 &-1 &-1 &-1 &-1 &-1 &-1 &-1 \\
\bottomrule
\end{tabular}
\end{table*}
\input{tables/table03.tex}
